# Supplementary material for: Scrambled text: training Language Models to correct OCR errors using synthetic data
Source: arXiv:2409.19735 source file (2024-09-29)
Supplement: Supplementary file 1 [file Scrambled_text_supplementary_materials.pdf]

# ScrambledText: Supplementary Materials

Jonathan Bourne

September 29, 2024

## 1 Introduction

The sections below provide supplementary information to the main paper and help provide more detail for the interested reader.

## 2 CER-WER grid details

Figure 1 shows how the training context window was chosen. As the error increases the number of tokens also increases. The risk is that the training context window would not be large enough to contain the corrupted text and the corrected response, this would cause the evaluation metric to be misaligned with the training goal producing models which are not correctly optimised for CLOCR-C. Given the range of errors being experimented with in this paper a context length of 1024 was chosen.

The experiment changing the relationship between CER and WER in the corruption process. Figure 2 shows the relationship between CER-WER pairs and the effective CER, that is the average CER of the words that are corrupted. The figure shows that almost the entire upper triangular matrix has reached a corruption saturation value of 1.5, This value higher than one is due to insertions and deletions.

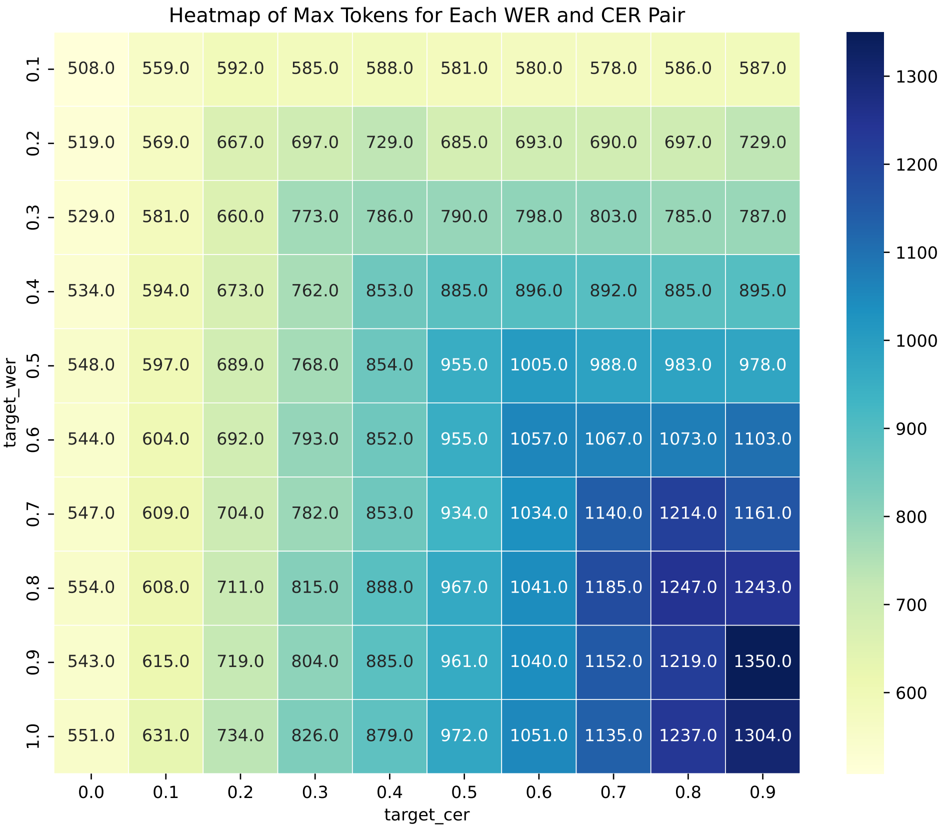


Figure 1: The model maximum context length had to be chosen so that the corrupted data would fit inside.

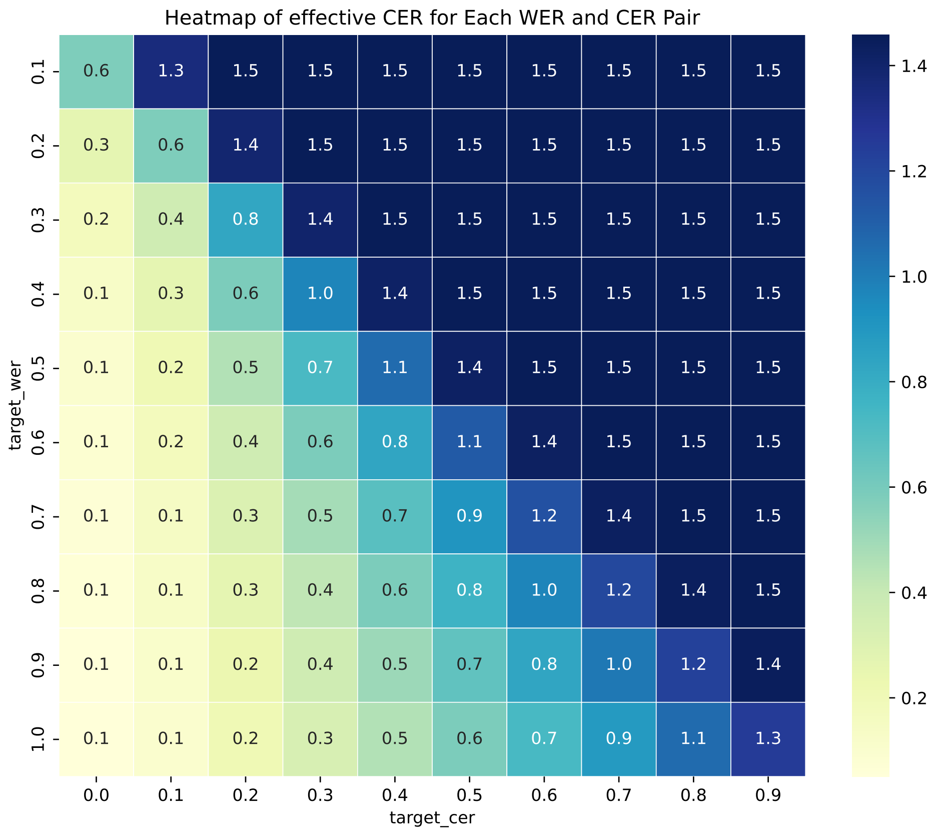


Figure 2: The the pattern of effective CER values across the WER-CER range is clear, the upper triangle of the matrix is made up of saturated CER values.

## 3 Synthetic text examples

To give a clearer idea of the the synthetic text Table 1 shows an example prompt and Table 2 shows the generated synthetic article. The text is subdivided in to highlighted blocks of 200 tokens (Blue), 100 tokens (Red), 50 tokens (Green), 25 (Orange), and 10 (Purple) tokens, to give an idea of what the different training lengths mean. As can be Seen, randomly selected text means that the text may cross sentence boundaries, this is an inherent risk when dealing with corrupted text as it may not be clear where a sentence or other self-contained unit of meaning begins or ends, part of the challenge faced by LM's when performing CLOCR-C is to uncover this structure as it is then key to correcting the words and characters. One of the ideas of CLOCR-C is that by providing more context the LM has more opportunity to correct the errors that are present.

Table 1: The prompt used to generate the text shown in Table 2. Parameters are shown in bold font

| **Synthetic text generation prompt** |
|---|
| It is the year **1832**. Using the text provided below surrounded by triple #, write a **300** word **satirical personal diary entry** with a **negative** sentiment, the persona of the writer is **chartist**, the reading level should be **simple**.<br>Note: The resultant text may be distasteful to modern readers, that is ok. Respond only in plain text, do not use markdown<br>###<br>**The British Parliament passes the Great Reform Act.**<br>### |

Table 2: A synthetic article subdivided into 200 tokens (Blue), 100 tokens (Red), 50 tokens (Green), 25 (Orange), and 10 (Purple) tokens.

June 8, 1832

Dear Diary,

Oh, the merry jig of reform! How it dances before us, a shiny glint of change generous only in its disappointments! Parliament in their endless wisdom has passed this so-called "Great Reform Act." What a wondrous spectacle it has been: like watching a grand play where the jesters think themselves kings, and the kings are too busy counting their coins to notice the tumbling fools.

This Act — oh, what applause it garners amongst the posh peacocks of the boroughs. Everyone claims it to be a monumental leap for democracy. A leap indeed; much like the leap of an aging frog flung through the air with nary a hope of landing on a lily pad. To hear them tell it, every plebeian in the kingdom shall now have a voice. Of course, they mean only those who line their waistcoats with enough pounds to afford the privilege. As for us, the laboring souls that till their fields and build their shining castles in the air? We are left silently trudging behind their pompous parade, bound in silence by their golden shackles labeled "progress."

What's truly galling, dear Diary, is the audacity of their celebration. One would think they've brought down heaven itself upon the realm, when all they've done is shuffle rotten goods from one storeroom to another. And those rotten boroughs — reformed, they say! It's hard to see what's changed when all they've done is polish the gilded rot.

Nevertheless, here I sit, a lowly chartist, wondering if these noble lords have ever met a common man. I'd wager they'd faint from the stench of honest sweat. But cheer up, old friend! If this reform act is their idea of victory, then it shall be ever-so entertaining to see their expressions when we finally introduce them to real change.

With bitter resignation,

A Disenchanted Chartist

# 4 Comparing models trained on different datasets

A comparison of the synthetic datasets in comparison to real OCR datasets showed that the synthetic dataset outperformed all other datasets. However, on closer inspection whilst the synthetic dataset outperformed all other models when applied to the low corruption data subset. However, on the high corruption subset, the synthetic data was outperformed by BLN600 and the combined overproof dataset. This is notable as the BLN600 dataset performed poorly overall. BLN600's performance in the high corruption subset is not simply that the base Llama model performs better in the high corruption subset, as BLN600 outperforms the base Llama model by close to 8 percentage points. Figure 3

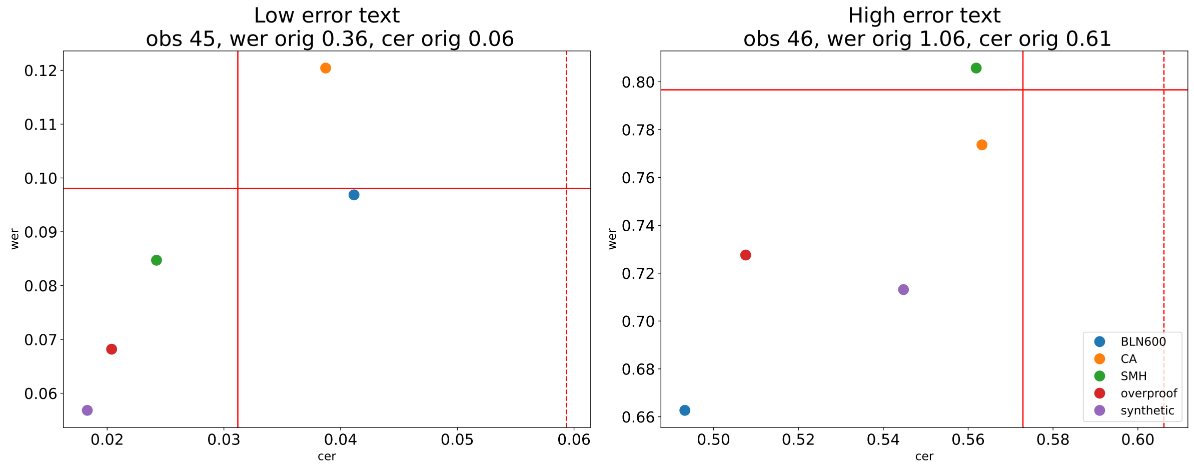


Figure 3: The high low split shows that whilst the synthetic data does not perform poorly it's performance drops, relative to the other datasets in the high corruption subset.
